# Supplementary material for: Probing the limits of materials design via a comprehensive crystal database of 14.6 million structures with 140 properties
Source: arXiv:2610.32678 source file (2026-11-19)
Supplement: Supplementary file 1 [file si-xr.tex]

\makeatletter
\expandafter\gdef\csname r@si-fig:completion-sets\endcsname{{S3}{15}{\textbf {From registered properties to training sets.} (a) Of the 166 properties in the registry, 151 carry a value. Splitting them by level of theory gives 513 candidate tasks, of which 197 have at least 10{,}000 crystals, and 176 training sets were built from these. Only the separation by level of theory increases the number of candidate tasks. (b) Training sets per declared applicability domain. (c) Crystals in each set's declared domain against crystals that already carry a label. The dashed diagonal marks equality and the dotted line the 14{,}590{,}485 crystals of the database.\relax }{}{}}
\expandafter\gdef\csname r@si-fig:contents\endcsname{{S1}{14}{\textbf {Contents of the property layer.} \textbf {a},~Number of populated properties per structure, with grey marking structures without a recorded property value. The 10{,}780 structures with 46 to 83 recorded properties lie beyond the plotted range. \textbf {b},~Stored spectra and the distinct structures represented, grouped by curve type. \textbf {c},~Property coverage by database, for the most widely covered properties and the databases annotating the most structures. Marker area scales with the number of structures carrying that value, colour marks the database family, and their legends appear above the grid. Databases appear under short names here and under their keys in Table~\ref {tab:sources}. The CSLLM negatives row is empty because its one property lies outside the columns shown.\relax }{}{}}
\expandafter\gdef\csname r@si-fig:mlip-calibration\endcsname{{S7}{36}{\textbf {MatterSim and reference GGA elastic moduli.} \textbf {a},~Bulk modulus from MatterSim against the GGA label for 300 crystals, of which 200 were drawn at random (circles) and 100 from those labelled at 200~GPa or above (triangles). Twenty of the random draw are also labelled at 200~GPa or above. The black line is parity and the second solid line has the median ratio of MatterSim to label as its slope. Dashed lines mark the threshold of 250~GPa, and the numbers in the four quadrants count the crystals. \textbf {b},~Shear moduli for the 289 crystals with a recorded shear-modulus value, with the 150~GPa threshold of Prop.~1. One crystal lies below the axis and its value is printed.\relax }{}{}}
\expandafter\gdef\csname r@si-fig:novelty-holders\endcsname{{S6}{35}{\textbf {Source databases containing generated structures matched by fingerprint.} For each of the eleven sources with the most matches, the bar counts generated structures matched by criterion 1 (the structural fingerprint). The 3{,}806 crystals are pooled over the five released 500-structure samples (CDVAE, CrystaLLM, FTCP, ion exchange and random enumeration) and the two MatterGen runs generated here. Their matches are found against all 55 sources, as at the all-source point of main-text Fig.~\ref {main-fig:novelty}b, and a crystal recorded in several databases counts once for each. Materials Project, commonly used for novelty assessment, holds 19. All eleven are general-purpose DFT databases and take that family's colour from Fig.~\ref {main-fig:record}b of the main text. GNoME is not pooled, and of its 18{,}234 exact matches Alexandria holds 14{,}709 and Materials Project one.\relax }{}{}}
\expandafter\gdef\csname r@si-fig:parity\endcsname{{S2}{15}{\textbf {Predicted and reference formation energies.} The 5{,}572 crystals of the JARVIS-DFT test split, predicted by the configuration of Table~\ref {tab:gnn-config}. Colour gives the number of crystals in each hexagonal bin on a logarithmic scale, and the dashed line marks parity. Of these crystals, \WithinAgreeWindow {}\% lie within 50~meV/atom of parity and \WithinWorstPair {}\% within 205~meV/atom.\relax }{}{}}
\expandafter\gdef\csname r@si-fig:route-detail\endcsname{{S8}{37}{\textbf {Structure-level verification of the ranked candidate lists.} \textbf {a}--\textbf {d},~MatterSim bulk modulus against the prediction of the ranking model for every verified structure of the four top-100 lists: paradigm A (\textbf {a}), paradigm B (\textbf {b}), B-exp (\textbf {c}) and B-exp restricted post hoc to confirmed synthesis evidence (\textbf {d}). Each panel draws its own list in colour over the other three in grey. Circles are Born-stable and crosses Born-unstable, the solid line is parity and the dashed lines mark 250~GPa on both axes. One structure of B-exp is not drawn because its elastic tensor is all zero and hence singular, which leaves its bulk modulus undefined. \textbf {e},~Share of the structures of each list that contain Os, Re, Ir, W, C, B (boron) or N, taken over all 100 structures rather than over the candidates meeting the criteria as in Fig.~\ref {main-fig:novelty}e of the main text. The list colours are those of Fig.~\ref {main-fig:novelty}d,e.\relax }{}{}}
\expandafter\gdef\csname r@si-fig:task-accuracy\endcsname{{S5}{22}{\textbf {Held-out accuracy of the completion tasks.} Each row is one task, the rows are sorted by $R^2$ and set in two columns, and each label gives the property with its level of theory, condition or source in brackets. Bars give the held-out $R^2$, coloured by the calculation tier of the property (Table~\ref {tab:tiers}), and grey bars belong to properties without a tier. Dots give the nMAE on a logarithmic axis. The nMAE divides the held-out mean absolute error by the mean absolute deviation of the training labels. An nMAE of 1 corresponds to an error equal to the training-label dispersion. Dashed lines mark $R^2 = 0.5$ and 0.7 and an nMAE of 1. A dagger marks the two tasks trained on $\log (1+y)$, whose $R^2$ and nMAE are computed after predictions are converted back to physical target units. An asterisk marks a yes/no label trained as a regression target. VRH is the Voigt--Reuss--Hill average and EOS an equation-of-state fit. BVEL and BVSE are barriers from bond-valence energy landscapes and site energies, with 1D to 3D the dimension of the percolating path. SHG is second-harmonic generation, SLME the spectroscopic limited maximum efficiency and $\kappa $ the lattice thermal conductivity. Gas uptakes are grand-canonical values at the stated temperature and pressure, and Xe/Kr 20:80 is the binary mixture.\relax }{}{}}
\expandafter\gdef\csname r@si-fig:theory\endcsname{{S4}{16}{\textbf {One property name, several levels of theory.} For the most widely covered property names, the fraction of labels assigned to each level of theory. Colours mark the level of theory and are keyed below the bars. The badge in each bar marks the semilocal (GGA) level, which is the largest in every bar, and \emph {other} collects method strings that match no level. Meta-GGA reaches 4.4\% of the band-gap labels and uses the same grey as other hybrids, DFPT, GGA+U and GW-BSE, each of which stays below 0.2\% of every bar. The number beside each bar is the number of distinct levels associated with that property.\relax }{}{}}
\expandafter\gdef\csname r@si-note:agreement\endcsname{{S3}{10}{Cross-database redundancy and agreement}{}{}}
\expandafter\gdef\csname r@si-note:agreement-reading\endcsname{{S4}{13}{Reading the cross-database comparison}{}{}}
\expandafter\gdef\csname r@si-note:audit\endcsname{{S17}{41}{Completeness audit}{}{}}
\expandafter\gdef\csname r@si-note:census\endcsname{{S7}{13}{Census and construction of the training sets}{}{}}
\expandafter\gdef\csname r@si-note:completion\endcsname{{S9}{20}{Property-completion results}{}{}}
\expandafter\gdef\csname r@si-note:discussion\endcsname{{S15}{40}{Extended discussion}{}{}}
\expandafter\gdef\csname r@si-note:disorder\endcsname{{S13.5}{36}{Partially occupied entries}{}{}}
\expandafter\gdef\csname r@si-note:fingerprint\endcsname{{S1}{3}{Limits of structural-fingerprint matching}{}{}}
\expandafter\gdef\csname r@si-note:licence\endcsname{{S21}{48}{Licence handling and the ICSD position}{}{}}
\expandafter\gdef\csname r@si-note:limits\endcsname{{S16}{41}{Limitations}{}{}}
\expandafter\gdef\csname r@si-note:methods\endcsname{{S18}{42}{Extended Methods}{}{}}
\expandafter\gdef\csname r@si-note:methods-audit\endcsname{{S18.3}{42}{Audit}{}{}}
\expandafter\gdef\csname r@si-note:methods-census\endcsname{{S18.5}{43}{Census and training-set construction}{}{}}
\expandafter\gdef\csname r@si-note:methods-comparison\endcsname{{S18.4}{42}{Cross-database comparison}{}{}}
\expandafter\gdef\csname r@si-note:methods-completion\endcsname{{S18.7}{43}{Property completion}{}{}}
\expandafter\gdef\csname r@si-note:methods-identity\endcsname{{S18.2}{42}{Identity resolution}{}{}}
\expandafter\gdef\csname r@si-note:methods-model\endcsname{{S18.6}{43}{Property model and benchmarks}{}{}}
\expandafter\gdef\csname r@si-note:methods-novelty\endcsname{{S18.9}{45}{Novelty audit of generated structures}{}{}}
\expandafter\gdef\csname r@si-note:methods-route\endcsname{{S18.10}{45}{Equal-budget comparison}{}{}}
\expandafter\gdef\csname r@si-note:methods-screening\endcsname{{S18.8}{44}{Screening}{}{}}
\expandafter\gdef\csname r@si-note:methods-sources\endcsname{{S18.1}{42}{Sources and their ingestion}{}{}}
\expandafter\gdef\csname r@si-note:mlip\endcsname{{S12}{31}{Verification by DFT and MatterSim}{}{}}
\expandafter\gdef\csname r@si-note:model\endcsname{{S8}{17}{The property model in detail}{}{}}
\expandafter\gdef\csname r@si-note:novelty\endcsname{{S13}{34}{The novelty audit in full}{}{}}
\expandafter\gdef\csname r@si-note:occupancy\endcsname{{S5}{13}{Occupancy of the crystal--property matrix}{}{}}
\expandafter\gdef\csname r@si-note:order\endcsname{{S2}{3}{Ingestion order and re-running sources}{}{}}
\expandafter\gdef\csname r@si-note:pipeline\endcsname{{S19}{46}{The integration pipeline}{}{}}
\expandafter\gdef\csname r@si-note:prereg\endcsname{{S10}{21}{Pre-registration and deviations}{}{}}
\expandafter\gdef\csname r@si-note:provenance\endcsname{{S20}{47}{Provenance and the canonical property registry}{}{}}
\expandafter\gdef\csname r@si-note:route\endcsname{{S14}{37}{Forward screening and inverse design at an equal verification budget}{}{}}
\expandafter\gdef\csname r@si-note:screening\endcsname{{S11}{29}{Screening predicted properties for four functional targets}{}{}}
\expandafter\gdef\csname r@si-note:tiers\endcsname{{S6}{13}{Calculation-tier assignment}{}{}}
\expandafter\gdef\csname r@si-si:gnn\endcsname{{S8}{18}{The property model in detail}{}{}}
\expandafter\gdef\csname r@si-tab:completion-tasks\endcsname{{S9}{23}{\textbf {The 140 property-prediction tasks.} A task specifies a property, level of theory and, where relevant, condition. Released task identifiers join the property name and theory level with a double underscore. \emph {Labels} counts structures with recorded values, which are excluded from prediction. \emph {Predicted} counts one value per unlabelled structure within the applied domain. Coverage is the fraction of 14{,}590{,}485 database structures with recorded values before completion and recorded or predicted values afterwards. Whole chemical systems are held out, and the actual structure count is listed for each task. The nMAE divides held-out MAE by the mean absolute deviation of the training labels about their mean. A dagger marks the two tasks trained on $\log (1+y)$, whose MAE and nMAE are computed after converting predictions back to physical target units. An asterisk marks binary labels treated as regression targets. A double dagger marks the four tasks for which the available data cannot fully enforce the declared domain. Their predicted counts and coverage are upper bounds (Note~\ref {note:completion}). Dashes mark unavailable quantities or dimensionless units.\relax }{}{}}
\expandafter\gdef\csname r@si-tab:db-numbers\endcsname{{S2}{12}{\textbf {Source numbering in Fig.~\ref {main-fig:record}b.} The 55 databases are numbered in descending order of their contributed property-value counts, with the largest assigned 1. \emph {Values} gives this count. Names match those in the figures and text.\relax }{}{}}
\expandafter\gdef\csname r@si-tab:dft-settings\endcsname{{S13}{33}{\textbf {DFT settings by stage.} All stages use PBE with the projector augmented-wave potentials of the Materials Project in VASP 6.3, \texttt {PREC = Accurate}, aspherical gradient corrections inside the augmentation spheres (\texttt {LASPH}), projection in reciprocal space (\texttt {LREAL = .FALSE.}) and $\Gamma $-centred $k$-point grids. Spin polarization and DFT+$U$ follow the rules of Note~\ref {note:mlip}, and the strained cells use the $k$-point grid of the relaxed cell. Dashes mark settings that do not apply.\relax }{}{}}
\expandafter\gdef\csname r@si-tab:gnn-config\endcsname{{S6}{19}{\textbf {CGTNet configuration for the JARVIS-DFT benchmarks.} Values are taken from the \texttt {resolved\_config.json} of the run that produced the formation-energy result in Table~\ref {tab:gnn-jarvis}. The same configuration is used for all four JARVIS-DFT properties. The MBJ band-gap run uses a denser prebuilt graph with 43.3 edges per atom. Edges per atom are measured from the prebuilt graphs.\relax }{}{}}
\expandafter\gdef\csname r@si-tab:gnn-jarvis\endcsname{{S7}{20}{\textbf {JARVIS-DFT benchmark errors.} Mean absolute errors on the standard test split. The CGTNet results use a common configuration, with a denser neighbour graph for the MBJ band gap, and are compared with published results compiled for this work. The lowest value in each column is bold.\relax }{}{}}
\expandafter\gdef\csname r@si-tab:gnn-matbench\endcsname{{S8}{20}{\textbf {Matbench benchmark errors.} Mean absolute errors over the five official folds. CGTNet uses task-specific settings (Note~\ref {note:methods-model}). Other values are published results or leaderboard submissions. The lowest value in each column is bold.\relax }{}{}}
\expandafter\gdef\csname r@si-tab:pairs\endcsname{{S3}{4}{\textbf {Pairwise agreement between databases.} Each row gives a database pair sharing at least 200 structures for a comparable property. $\Delta $ is the difference in the listed database order. Similar median signed and absolute differences indicate predominantly one-sided differences, consistent with a systematic offset.\relax }{}{}}
\expandafter\gdef\csname r@si-tab:properties\endcsname{{S4}{7}{\textbf {The 151 properties with recorded values.} Properties are ordered by the number of structures with values. \emph {Sources} counts databases reporting the property, and \emph {Shared} counts structures with values from at least two databases irrespective of theory level. The main-text agreement analysis uses smaller subsets restricted to comparable theory levels (Note~\ref {note:agreement}).\relax }{}{}}
\expandafter\gdef\csname r@si-tab:route\endcsname{{S14}{38}{\textbf {Verification of generated and screened candidates.} MatterSim evaluates the 100 highest-ranked structures in each list. The number evaluated by DFT is given separately. The right block retains one structure per reduced formula, as specified in the pre-registered secondary analysis. Paradigm A contains MatterGen structures generated with a 400~GPa bulk-modulus condition. Paradigm B contains database structures without a recorded bulk modulus, and B-exp is its experimental-source subset. Candidates satisfy the verification criteria when their bulk modulus is at least 250~GPa and their elastic tensor is Born-stable. DFT rows apply these criteria to the PBE tensors described in Note~\ref {note:mlip}. Other rows report MatterSim results. Unless indicated otherwise, composition, diversity and property statistics refer to candidates meeting these criteria. The ranking model has a held-out RMSE of 15.2~GPa. Each list is compared with paradigm A in the same block using a two-sided Fisher exact test on criterion satisfaction and a two-sided Mann--Whitney test on Born-stable MatterSim bulk moduli. Duplicates match labelled structures under the stated StructureMatcher tolerances. Novelty rows apply the four criteria in Note~\ref {note:novelty} to generated candidates meeting the verification criteria. Hardware differs: generation used one RTX 4080 Laptop GPU and property inference used RTX 4090 D GPUs. Paradigm B's cost includes both consecutive inference processes over the full domain. The literal pre-registered cost includes only the last process, whose time was stored with the predictions (Note~\ref {note:route}). Dashes mark inapplicable quantities.\relax }{}{}}
\expandafter\gdef\csname r@si-tab:route-variants\endcsname{{S15}{40}{\textbf {Post hoc variants of screening paradigm B.} S restricts B-exp to structures with synthesis evidence. T removes structures matched by StructureMatcher to entries with a bulk-modulus value and fills each list from lower ranks until it contains 100 structures. T$'$ applies the same procedure without removing oxidation-state labels before species comparison. Each list is compared with the corresponding paradigm-A list, either the top 100 or one structure per formula. \emph {Depth} gives the lowest rank required to fill the list. \emph {Gap} is the difference between the maximum verified bulk moduli of the listed set and paradigm A. The two \emph {Number} columns count Born-stable candidates at or above 250 and 200~GPa. \emph {Chem. systems} counts their chemical systems at 250~GPa, and e$_\mathrm {hull}$ gives the fraction within 0.1~eV/atom of the MatterSim hull. Maximum moduli are considered different only when their gap exceeds the 41.2~GPa MatterSim calibration error above 300~GPa (Note~\ref {note:mlip}). The final columns identify the paradigm favoured by the fraction meeting the criteria (two-sided Fisher test), maximum modulus, and distribution of Born-stable moduli (two-sided Mann--Whitney test). An equals sign indicates no difference under the specified rule. Paradigm A has the larger fraction in all 18 comparisons. Outcome~1 applies to one list, with a margin of 0.48~GPa on the maximum-modulus criterion. No pre-declared outcome applies to the other lists.\relax }{}{}}
\expandafter\gdef\csname r@si-tab:screening-attrition\endcsname{{S11}{32}{\textbf {Candidates remaining after each post hoc audit rule.} Each cell gives the number of remaining structures, with the number of chemical systems in brackets. Rules are applied in the listed order. A dash marks a rule that does not apply. The upper block starts from the pre-registered selection set in Table~\ref {tab:screening-counts}, while the lower block starts from all candidates. For Prop.~4, the lower block includes the additional inference under rule 5 and therefore starts with 8{,}754 candidates rather than the pre-registered 3{,}525. After rule 4, the lower block contains the audited candidates without a compound-level primary-property record. Both blocks end with the same subset supported by synthesis evidence. The rules were fixed after the literature check of the pre-registered selections and before any audited result was computed (Note~\ref {note:prereg}). An independent recount reproduced every set.\relax }{}{}}
\expandafter\gdef\csname r@si-tab:screening-counts\endcsname{{S10}{32}{\textbf {Results of the pre-registered screen.} Counts use the definitions fixed before candidate enumeration (Note~\ref {note:prereg}). A structure is eligible when every criterion has either a recorded value at the selected level of theory or a model prediction. The primary property is bulk modulus for Prop.~1, migration barrier for Prop.~2, voltage for Prop.~3 and birefringence for Prop.~4. \emph {No recorded primary value} means that no integrated source reports that property for the selected structure at any level of theory. A predicted primary value can coexist with a recorded value under another name or level. This excludes 1{,}140 Prop.~1 candidates and 6 Prop.~4 candidates from the no-record category. Experimental-source structures are the 357{,}127 structures from experimental structure databases, as defined in the original pre-registration. Recorded hull distances are reported separately and are not used to filter candidates. An independent recount reproduced every count.\relax }{}{}}
\expandafter\gdef\csname r@si-tab:showcase\endcsname{{S12}{30}{\textbf {Selected candidates and literature evidence.} For each target, the pre-registered selection comprises the three highest-ranked candidates from distinct chemical systems among experimental-source structures without a recorded primary-property value. The same rule is applied to candidates with synthesis evidence in the post hoc audit. Prop.~2 has no audited selection. \emph {Entry} identifies the source record. \emph {Primary} and \emph {second} give the predicted primary property and the secondary-criterion value. \emph {MS} gives the MatterSim bulk modulus for Prop.~1 (Note~\ref {note:mlip}), with superscript u marking a Born-unstable tensor. The final column summarises the literature check and the audit rules failed by the original selections (Table~\ref {tab:screening-attrition}). Literature findings were reported but were not used to include or exclude candidates.\relax }{}{}}
\expandafter\gdef\csname r@si-tab:sources\endcsname{{S1}{11}{\textbf {The 55 integrated source databases.} Counts describe property values, distinct properties and structures represented in the assembled database. \emph {Matched} references are resolved by identifier or fingerprint. \emph {Own} references indicate that the source contains a corresponding entry, which need not mean it contributed the structure. Licence categories follow the provider audit. A dagger marks the 18 sources that prohibit redistribution, permit only non-commercial redistribution or provide no clear licence (Note~\ref {note:licence}).\relax }{}{}}
\expandafter\gdef\csname r@si-tab:tiers\endcsname{{S5}{12}{\textbf {Computational-cost tiers for 69 general-purpose properties.} The manual assignment reflects the calculations required for each property and is listed in full for inspection. The other 82 populated properties are excluded, including structural descriptors, calculation metadata and properties defined for a single material family (Note~\ref {note:tiers}).\relax }{}{}}
\makeatother
